# Supplementary material for: Clues Before Answers: Generation-Enhanced Multiple-Choice QA
Source: arXiv:2205.00274 source file (2022-04-30)
Supplement: Supplementary file 1 [file 7-appendix.tex]

\section{Appendix}
\label{sec:Appendix}

\begin{table*}[t!]
\centering
% \small
\resizebox{\textwidth}{!}{$
% \resizebox{\columnwidth}{!}{$
\begin{tabular}{lccccccccccc}
% \begin{tabular}{llllllllllll}
\hline
& \multicolumn{2}{c}{CSQA} & \multicolumn{2}{c}{OBQA} & \multicolumn{2}{c}{ARC-Easy} & \multicolumn{2}{c}{ARC-Challenge} & \multicolumn{2}{c}{QASC} \\
\cline{2-11}
& dev & test & dev & test & dev & test  & dev & test  & dev & test \\
\hline
BART$_\text{base}$ \\
\quad Text2Text$_\text{vanilla}$ & 51.62~($\pm$0.04) & 53.26~($\pm$0.57) & 54.93~($\pm$0.83) & 52.73~($\pm$1.00) &  51.55~($\pm$1.38) & 50.51~($\pm$1.82) & 30.05~($\pm$1.25) & 24.95~($\pm$ 1.10) & 46.72~($\pm$1.21) & 26.78~($\pm$1.21)   \\

\quad Text2Text$_\text{Enc}$ & 50.63~($\pm$0.66) & 52.22~($\pm$1.64) & 55.87~($\pm$1.10) &  51.00~($\pm$1.83) & 49.03~($\pm$1.86) & 49.94~($\pm$1.49) & 32.32~($\pm$4.87) & 26.24~($\pm$2.01) & 48.08($\pm$1.35) & 17.06~($\pm$0.39) \\

\quad Our Model & \textbf{54.82~($\pm$0.61)} & \textbf{56.40}~($\pm$0.61) & \textbf{58.53}~($\pm$0.31) &  \textbf{57.53}~($\pm$2.91) & \textbf{59.38}~($\pm$1.60) & \textbf{56.80}~($\pm$0.28) & \textbf{38.64}~($\pm$0.90) & \textbf{33.82}~($\pm$1.66) & \textbf{57.70}~($\pm$0.43) & \textbf{35.96}~($\pm$1.70) \\

\hline
T5$_\text{base}$ \\
\quad Text2Text$_\text{vanilla}$ & 57.59~($\pm$0.81) & 60.93~($\pm$0.73) & 59.53~($\pm$0.81) &  57.53~($\pm$0.70) & 52.20~($\pm$0.31) & 51.75~($\pm$0.89) & 29.38~($\pm$2.63) & 23.69~($\pm$2.47) & 54.55~($\pm$1.01) & 37.94~($\pm$1.47)   \\
\quad Text2Text$_\text{Enc}$ & 58.96~($\pm$1.21) & 59.49~($\pm$1.41) & 60.67~($\pm$2.86) &  57.07~($\pm$3.03) & 56.55~($\pm$1.17) & 52.92~($\pm$0.29) & 29.49~($\pm$5.13) & 26.09~($\pm$0.23) & 56.84~($\pm$0.84) & 39.60~($\pm$2.38)   \\
\quad Our Model & \textbf{60.65}~($\pm$0.47) & \textbf{63.45}~($\pm$0.29) & \textbf{
62.07}~($\pm$1.01) &  \textbf{61.67}~($\pm$0.58) & \textbf{62.38}~($\pm$0.67) & \textbf{58.82}~($\pm$0.37) & \textbf{43.62}~($\pm$0.52) & \textbf{
39.00}~($\pm$0.30) & \textbf{58.93}~($\pm$1.76) & \textbf{41.72}~($\pm$1.18)  \\
\hline

BART$_\text{large}$ \\
\quad Text2Text$_\text{vanilla}$ & 65.58~($\pm$2.72) & 66.91~($\pm$2.14) & 62.66~($\pm$1.18) &  61.46~($\pm$1.74) & 63.49~($\pm$1.89) & 62.81~($\pm$2.15) & 29.94~($\pm$2.32) & 28.55~($\pm$4.97) & 64.57~($\pm$2.21) & 47.80~($\pm$2.22)  \\

\quad Text2Text$_\text{Enc}$ & 65.00~($\pm$0.66) & 67.35~($\pm$0.90) & 63.80~($\pm$1.44) &  62.47~($\pm$1.53) & 68.20~($\pm$2.04) & 65.33~($\pm$1.74) & 35.37~($\pm$6.07) & 31.13~($\pm$5.86) & 65.07~($\pm$0.94) & 47.19~($\pm$0.71)  \\

\quad Our Model & \textbf{69.57}~($\pm$0.89) & \textbf{72.26}~($\pm$0.70) & \textbf{68.93}~($\pm$1.17) &  \textbf{68.07}~($\pm$1.70) & \textbf{72.43}~($\pm$0.54) & \textbf{68.68}~($\pm$0.34) &\textbf{48.93}~($\pm$0.98) & \textbf{45.52}~($\pm$1.54) & \textbf{68.39
}~($\pm$0.68) & \textbf{55.90}~($\pm$0.92)  \\
\hline

T5$_\text{large}$ \\
\quad Text2Text$_\text{vanilla}$ & 67.53~($\pm$0.43) & 70.63~($\pm$0.74) & 66.80~($\pm$0.87) &  63.53~($\pm$1.10) & 65.61~($\pm$0.18) & 62.55~($\pm$0.54) & 43.05~($\pm$1.69) & 42.83~($\pm$2.00) & 64.13~($\pm$1.47) & 57.74~($\pm$0.82)  \\

\quad Text2Text$_\text{Enc}$ & 68.41~($\pm$0.73) & 70.30~($\pm$0.82) & 65.93~($\pm$1.03) &  63.67~($\pm$0.46) & 69.61~($\pm$0.20) & 66.65~($\pm$0.34) & 30.73~($\pm$3.15) & 28.76~($\pm$4.85) & 65.27~($\pm$1.55) & 55.65~($\pm$0.45)   \\

\quad Our Model & \textbf{71.10}~($\pm$0.41) & \textbf{72.67}~($\pm$1.02) & \textbf{71.60}~($\pm$0.92) &  \textbf{66.87}~($\pm$1.33) & \textbf{72.49}~($\pm$0.77) & \textbf{69.01}~($\pm$1.97) & \textbf{49.83}~($\pm$2.06) & \textbf{47.41}~($\pm$2.00) & \textbf{67.61}~($\pm$1.14) & \textbf{58.06}~($\pm$0.92)  \\
\hline
\end{tabular}
$}

\caption{Improvements to the Text-to-Text model.}
\label{table:comp_t2t_model}
\end{table*}

\begin{table*}[t!]
\centering
% \small
\resizebox{\textwidth}{!}{$
% \resizebox{\columnwidth}{!}{$
\begin{tabular}{lccccccccccc}
\hline
& \multicolumn{2}{c}{CSQA} & \multicolumn{2}{c}{OBQA} & \multicolumn{2}{c}{ARC-Easy} & \multicolumn{2}{c}{ARC-Challenge} & \multicolumn{2}{c}{QASC} \\
\cline{2-11}
& dev & test & dev & test & dev & test  & dev & test  & dev & test \\
\hline
BART$_\text{base}$ \\
\quad Our Model & \textbf{54.82~($\pm$0.61)} & \textbf{56.40}~($\pm$0.61) & \textbf{58.53}~($\pm$0.31) &  \textbf{57.53}~($\pm$2.91) & \textbf{59.38}~($\pm$1.60) & \textbf{56.80}~($\pm$0.28) & 38.64~($\pm$0.90) & \textbf{33.82}~($\pm$1.66) & \textbf{57.70}~($\pm$0.43) & \textbf{35.96}~($\pm$1.70) \\
\quad w/o gen loss & 53.96~($\pm$1.01) & 54.35~($\pm$1.97) & 55.53~($\pm$1.27) &  54.27~($\pm$0.92) & 57.20~($\pm$1.80) & 55.42~($\pm$1.26) & \textbf{39.89}~($\pm$0.20) & 32.62~($\pm$0.31) & 54.05~($\pm$0.21) & 25.99~($\pm$0.82)  \\  
\quad w/o clue & 53.67~($\pm$0.58) & 54.30~($\pm$0.83) & 55.60~($\pm$0.72) &  53.60~($\pm$2.62) & 56.91~($\pm$0.71) & 54.90~($\pm$0.58) & 37.63~($\pm$1.48) & 32.27~($\pm$0.26) & 54.26~($\pm$1.11) & 26.67~($\pm$0.71)  \\  
\hline

T5$_\text{base}$ \\
\quad Our Model & \textbf{60.65}~($\pm$0.47) & \textbf{63.45}~($\pm$0.29) & \textbf{
62.07}~($\pm$1.01) &  \textbf{61.67}~($\pm$0.58) & \textbf{62.38}~($\pm$0.67) & \textbf{58.82}~($\pm$0.37) & \textbf{43.62}~($\pm$0.52) & \textbf{
39.00}~($\pm$0.30) & \textbf{58.93}~($\pm$1.76) & \textbf{41.72}~($\pm$1.18)  \\
\quad w/o gen loss & 58.80~($\pm$0.70) & 60.88~($\pm$1.89) & 61.47~($\pm$0.95) &  59.73~($\pm$0.90) & 58.97~($\pm$0.54) & 57.10~($\pm$0.72) & 42.26~($\pm$2.21) & 37.54~($\pm$0.64) & 57.37~($\pm$1.40) & 36.29~($\pm$1.66)  \\  
\quad w/o clue & 58.55~($\pm$0.40) & 59.05~($\pm$0.71) & 61.60~($\pm$0.53) &  58.27~($\pm$2.05) & 60.32~($\pm$2.37) & 56.84~($\pm$1.78) & 38.87~($\pm$2.54) & 36.25~($\pm$1.73) & 58.07~($\pm$1.42) & 36.36~($\pm$0.92)  \\  
\hline

BART$_\text{large}$ \\
\quad Our Model & \textbf{69.57}~($\pm$0.89) & \textbf{72.26}~($\pm$0.70) & \textbf{68.93}~($\pm$1.17) &  \textbf{68.07}~($\pm$1.70) & 72.43~($\pm$0.54) & \textbf{68.68}~($\pm$0.34) &\textbf{48.93}~($\pm$0.98) & \textbf{45.52}~($\pm$1.54) & \textbf{68.39
}~($\pm$0.68) & \textbf{55.90}~($\pm$0.92)  \\
\quad w/o gen loss & 67.28~($\pm$2.39) & 69.64~($\pm$2.76) & 66.20~($\pm$0.53) &  64.47~($\pm$1.40) & 70.66~($\pm$1.50) & 65.71~($\pm$1.47) & 27.80~($\pm$2.06) & 24.92~($\pm$2.06) & 65.68~($\pm$1.31) & 52.02~($\pm$1.44)  \\  
\quad w/o clue   & 68.95~($\pm$0.97) & 71.61~($\pm$1.07) & 66.87~($\pm$0.12) &  65.40~($\pm$1.39) & \textbf{72.93}~($\pm$1.12) & 67.04~($\pm$0.69) & 46.67~($\pm$1.37) & 42.63~($\pm$1.01) & 67.16~($\pm$0.26) & 51.94~($\pm$1.31)  \\  
\hline

T5$_\text{large}$ \\
\quad Our Model & \textbf{71.10}~($\pm$0.41) & \textbf{72.67}~($\pm$1.02) & \textbf{71.60}~($\pm$0.92) &  \textbf{66.87}~($\pm$1.33) & \textbf{72.49}~($\pm$0.77) & \textbf{69.01}~($\pm$1.97) & \textbf{49.83}~($\pm$2.06) & \textbf{47.41}~($\pm$2.00) & \textbf{67.61}~($\pm$1.14) & \textbf{58.06}~($\pm$0.92)  \\
\quad w/o gen loss & 68.33~($\pm$1.62) & 71.66~($\pm$1.28) & 69.27~($\pm$0.42) &  65.87~($\pm$0.90) & 69.66~($\pm$0.77) & 66.24~($\pm$0.79) & 47.57~($\pm$2.04) & 46.24~($\pm$1.29) & 64.99~($\pm$0.74) & 53.35~($\pm$1.35)  \\  
\quad w/o clue & 67.79~($\pm$0.95) & 70.52~($\pm$0.22) & 69.40~($\pm$1.44) &  66.20~($\pm$0.72) & 67.61~($\pm$4.35) & 66.19~($\pm$3.40) & 45.08~($\pm$1.48) & 43.23~($\pm$0.95) & 65.52~($\pm$0.43) & 51.98~($\pm$1.68)   \\
\hline
\end{tabular}
$}
\caption{Influence of Clue.}
\label{table:wo_clue}
\end{table*}

\begin{table*}[t!]
\centering
% \small
\resizebox{\textwidth}{!}{$
% \resizebox{\columnwidth}{!}{$
\begin{tabular}{lccccccccccc}
\hline
& \multicolumn{2}{c}{CSQA} & \multicolumn{2}{c}{OBQA} & \multicolumn{2}{c}{ARC-Easy} & \multicolumn{2}{c}{ARC-Challenge} & \multicolumn{2}{c}{QASC} \\
\cline{2-11}
& dev & test & dev & test & dev & test  & dev & test  & dev & test \\
\hline
BART$_\text{base}$ \\
\quad Our Model & \textbf{54.82~($\pm$0.61)} & \textbf{56.40}~($\pm$0.61) & \textbf{58.53}~($\pm$0.31) &  \textbf{57.53}~($\pm$2.91) & \textbf{59.38}~($\pm$1.60) & \textbf{56.80}~($\pm$0.28) & \textbf{38.64}~($\pm$0.90) & \textbf{33.82}~($\pm$1.66) & \textbf{57.70}~($\pm$0.43) & \textbf{35.96}~($\pm$1.70) \\
\quad Pipeline Clue & 45.53~($\pm$1.28)  & 46.41~($\pm$1.79)   & 54.07~($\pm$1.72)  & 52.93~($\pm$1.1)  & 48.97~($\pm$0.91)  & 48.87~($\pm$1.29)  & 31.19~($\pm$0.59)  & 27.64~($\pm$0.69)  & 49.06~($\pm$0.39)  & 21.31~($\pm$1.03)  \\  
\hline

T5$_\text{base}$ \\
\quad Our Model & \textbf{60.65}~($\pm$0.47) & \textbf{63.45}~($\pm$0.29) & \textbf{
62.07}~($\pm$1.01) &  \textbf{61.67}~($\pm$0.58) & \textbf{62.38}~($\pm$0.67) & \textbf{58.82}~($\pm$0.37) & \textbf{43.62}~($\pm$0.52) & \textbf{
39.00}~($\pm$0.30) & \textbf{58.93}~($\pm$1.76) & \textbf{41.72}~($\pm$1.18)  \\
\quad Pipeline Clue & 50.55~($\pm$0.44)  & 48.79~($\pm$0.87) & 56.00~($\pm$1.25)  & 54.93~($\pm$1.63)  & 46.50~($\pm$0.83)  & 46.65~($\pm$0.54)  & 32.66~($\pm$0.20)  & 26.01~($\pm$1.28)  & 43.69~($\pm$1.52)  & 27.50~($\pm$1.56)  \\  

\hline
BART$_\text{large}$ \\
\quad Our Model & \textbf{69.57}~($\pm$0.89) & \textbf{72.26}~($\pm$0.70) & \textbf{68.93}~($\pm$1.17) &  \textbf{68.07}~($\pm$1.70) & \textbf{72.43}~($\pm$0.54) & \textbf{68.68}~($\pm$0.34) &\textbf{48.93}~($\pm$0.98) & \textbf{45.52}~($\pm$1.54) & \textbf{68.39
}~($\pm$0.68) & \textbf{55.90}~($\pm$0.92)  \\
\quad Pipeline Clue & 53.85~($\pm$0.47)  & 55.23~($\pm$0.62)   & 61.20~($\pm$3.14)  & 59.20~($\pm$0.69)  & 58.02~($\pm$0.98)  & 54.22~($\pm$1.27)  & 41.81~($\pm$1.19)  & 37.60~($\pm$0.90)  & 48.65~($\pm$1.23)  & 32.47~($\pm$1.11)  \\  
\hline
T5$_\text{large}$ \\
\quad Our Model & \textbf{71.10}~($\pm$0.41) & \textbf{72.67}~($\pm$1.02) & \textbf{71.60}~($\pm$0.92) &  \textbf{66.87}~($\pm$1.33) & \textbf{72.49}~($\pm$0.77) & \textbf{69.01}~($\pm$1.97) & \textbf{49.83}~($\pm$2.06) & \textbf{47.41}~($\pm$2.00) & \textbf{67.61}~($\pm$1.14) & \textbf{58.06}~($\pm$0.92)  \\
\quad Pipeline Clue & 59.47~($\pm$0.08)  & 60.74~($\pm$0.29)   & 62.80~($\pm$1.44)  & 57.73~($\pm$1.1)  & 48.85~($\pm$1.62)  & 48.36~($\pm$2.15)  & 37.97~($\pm$0.90)  & 30.50~($\pm$1.46)  & 49.22~($\pm$0.62)  & 38.77~($\pm$1.74)  \\  
\hline
\end{tabular}
$}
\caption{Influence of Clue Usage.}
\label{table:pipeline}
\end{table*}

\begin{table*}[t!]
\centering
\small
\resizebox{\textwidth}{!}{$
% \resizebox{\columnwidth}{!}{$
\begin{tabular}{lccccccccccc}
% \begin{tabular}{llllllllllll}
\hline
& \multicolumn{2}{c}{CSQA} & \multicolumn{2}{c}{OBQA} & \multicolumn{2}{c}{ARC-Easy} & \multicolumn{2}{c}{ARC-Challenge} & \multicolumn{2}{c}{QASC} \\
\cline{2-11}
& dev & test & dev & test & dev & test  & dev & test  & dev & test \\
\hline
base \\
\quad Roberta & 56.51~($\pm$0.34) & 58.91~($\pm$0.79) & 58.67~($\pm$1.03) &  49.67~($\pm$0.76) & 56.56~($\pm$0.91) & 52.32~($\pm$0.70) & 38.64~($\pm$0.90) & 34.85~($\pm$2.20) & 55.28~($\pm$(0.12) & 34.38~($\pm$1.72)  \\
\quad Albert & 53.16~($\pm$0.58) & 53.95~($\pm$0.49) & 54.53~($\pm$1.10) &  49.20~($\pm$2.27) & 48.32~($\pm$0.88) & 45.84~($\pm$1.94) & 34.80~($\pm$1.53) & 30.21~($\pm$1.74) & 40.99~($\pm$(1.78) & 24.55~($\pm$1.23)  \\
%\quad CALM~$\ast$ & - & 63.32~($\pm$0.35) & - &  60.90~($\pm$0.40) & - & - & - & - & - &\\
%\quad CALM & 54.83 & 56.68~($\pm$) & - &  ~($\pm$) & - & - & - & - & - &    \\
\quad UnifiedQA-T5~$\ast$ & 
- & 45.00~($\pm$0.00) & - &  59.00~($\pm$0.00) & - & 53.00~($\pm$0.00) & - & 42.40~($\pm$0.00) & - & 25.8~($\pm$0.00)    \\
\quad UnifiedQA-T5 & 41.02~($\pm$0.00) & 44.80~($\pm$0.00) & 59.20~($\pm$0.00) &  59.60~($\pm$0.00) & 54.85~($\pm$0.00) & 53.66~($\pm$0.00) & 44.75~($\pm$0.00) & 42.58~($\pm$0.00) & 17.94~($\pm$0.00) & 25.70~($\pm$0.00)  \\
\quad UnifiedQA-T5$_\text{finetune}$ & 56.81~($\pm$0.49) & 62.35~($\pm$0.80) & 60.80~($\pm$0.72) &  58.47~($\pm$0.64) & 54.97~($\pm$0.20) & 53.88~($\pm$0.39) & \textbf{45.31}~($\pm$0.39) & \textbf{42.43}~($\pm$0.47) & 55.57~($\pm$0.58) & \textbf{43.20}~($\pm$0.57)  \\
\quad Our Model & \textbf{60.65}~($\pm$0.47) & \textbf{63.45}~($\pm$0.29) & \textbf{
62.07}~($\pm$1.01) &  \textbf{61.67}~($\pm$0.58) & \textbf{62.38}~($\pm$0.67) & \textbf{58.82}~($\pm$0.37) & 43.62~($\pm$0.52) & 
39.00~($\pm$0.30) & \textbf{58.93}~($\pm$1.76) & 41.72~($\pm$1.18)  \\
\quad Our Model Unified& ~($\pm$) & ~($\pm$) & ~($\pm$) &  ~($\pm$) & ~($\pm$) & ~($\pm$)~($\pm$) & ~($\pm$) & ~($\pm$) & ~($\pm$) & ~($\pm$)  \\
\quad Our Model Unified$_\text{finetune}$ & ~($\pm$) & ~($\pm$) & ~($\pm$) &  ~($\pm$) & ~($\pm$) & ~($\pm$)~($\pm$) & ~($\pm$) & ~($\pm$) & ~($\pm$) & ~($\pm$)  \\
\hline

large \\
\quad Roberta & 68.92~($\pm$0.76) & 71.88~($\pm$0.26) & 67.80~($\pm$1.22) &  64.47~($\pm$1.41) & 65.73~($\pm$0.80) & 62.40~($\pm$0.89) & 38.08~($\pm$1.99) & 35.97~($\pm$1.74) & 67.73~($\pm$0.58) & 50.22~($\pm$1.88)  \\  
\quad ALBert & 60.62~($\pm$0.57) & 59.32~($\pm$0.91) & 54.50~($\pm$1.40) &  49.27~($\pm$0.64) & 54.03~($\pm$0.45) & 53.77~($\pm$1.81) & 33.90~($\pm$1.22) & 31.19~($\pm$3.79) & 51.11~($\pm$1.72) & 33.12~($\pm$1.24)  \\  
\quad CALM~$\ast$ & - & 71.31~($\pm$0.04) & - &  66.00~($\pm$1.00) & - & - & - & - & - &\\
\quad CALM & - & ~($\pm$) & - &  ~($\pm$) & - & - & - & - & - &    \\
\quad UnifiedQA-T5~$\ast$ & - & 60.90~($\pm$0.00) & - &  68.40~($\pm$0.00) & - & 65.90~($\pm$0.00) & - & 54.40~($\pm$0.00) & - & 43.30~($\pm$0.00)  \\
\quad UnifiedQA-T5 & 55.28~($\pm$0.00) & 61.34~($\pm$0.00) & 70.40~($\pm$0.00) &  68.40~($\pm$0.00) & 69.31~($\pm$0.00) & 66.43~($\pm$0.00) & 56.61~($\pm$0.00) & 54.33~($\pm$0.00) & 29.24~($\pm$0.00) & 43.74~($\pm$0.00)  \\
\quad UnifiedQA-T5$_\text{finetune}$ & 69.00~($\pm$0.51) & \textbf{73.60}~($\pm$0.45) & 70.53~($\pm$0.23) &  \textbf{68.80}~($\pm$0.69) & 69.72~($\pm$0.71) & \textbf{66.92}~($\pm$0.85) & \textbf{56.84}~($\pm$0.39) & \textbf{54.42}~($\pm$0.15) & 66.63~($\pm$1.56) & \textbf{58.71}~($\pm$0.90)  \\

\quad Our Model & \textbf{71.10}~($\pm$0.41) & 72.67~($\pm$1.02) & \textbf{71.60}~($\pm$0.92) &  66.87~($\pm$1.33) & \textbf{72.49}~($\pm$0.77) & \textbf{69.01}~($\pm$1.97) & 49.83~($\pm$2.06) & 47.41~($\pm$2.00) & \textbf{67.61}~($\pm$1.14) & 58.06~($\pm$0.92)  \\

\quad Our Model Unified& ~($\pm$) & ~($\pm$) & ~($\pm$) &  ~($\pm$) & ~($\pm$) & ~($\pm$)~($\pm$) & ~($\pm$) & ~($\pm$) & ~($\pm$) & ~($\pm$)  \\
\quad Our Model Unified$_\text{finetune}$& ~($\pm$) & ~($\pm$) & ~($\pm$) &  ~($\pm$) & ~($\pm$) & ~($\pm$)~($\pm$) & ~($\pm$) & ~($\pm$) & ~($\pm$) & ~($\pm$)  \\
\hline
% \quad Previous Best &
% -& 83.30& 
% -& 87.40&
% -& 94.78& 
% -& 86.52&
% -& 89.57
\quad UnifiedQA-T5-11B$_\text{finetune}$ &
-& 79.10& 
-& 86.00&
-& 86.40& 
-& 75.00&
-& 78.50
\\

\hline

\end{tabular}
$}
\caption{Comparison with Asymmetric Approach.}
\label{table:SOTA}
\end{table*}

%%%%%%%%%%%%%%%%%%%%%%%%%%%

\begin{table}[t!]
\centering
% \small
% \resizebox{\textwidth}{!}{$
\resizebox{\columnwidth}{!}{$
% \resizebox{\columnwidth}{!}{$
\begin{tabular}{cccccc}
\hline
& \multicolumn{1}{c}{CSQA} & \multicolumn{1}{c}{OBQA} & \multicolumn{1}{c}{ARC-Easy} & \multicolumn{1}{c}{ARC-Challenge} & \multicolumn{1}{c}{QASC} \\
\cline{2-11}
\hline
BART$_\text{base}$ \\
\quad Text2Text$_\text{vanilla}$ & 53.26~($\pm$0.57) & 52.73~($\pm$1.00)  & 50.51~($\pm$1.82)  & 24.95~($\pm$ 1.10) & 26.78~($\pm$1.21)   \\

\quad Text2Text$_\text{Enc}$ & 52.22~($\pm$1.64) &  51.00~($\pm$1.83)  & 49.94~($\pm$1.49)  & 26.24~($\pm$2.01) & 17.06~($\pm$0.39) \\

\quad Our Model & \textbf{56.40}~($\pm$0.61) &  \textbf{57.53}~($\pm$2.91) & \textbf{56.80}~($\pm$0.28)  & \textbf{33.82}~($\pm$1.66) & \textbf{35.96}~($\pm$1.70) \\

\hline

T5$_\text{base}$ \\
\quad Text2Text$_\text{vanilla}$  & 60.93~($\pm$0.73) &  57.53~($\pm$0.70) & 51.75~($\pm$0.89) & 23.69~($\pm$2.47)  & 37.94~($\pm$1.47)   \\
\quad Text2Text$_\text{Enc}$ & 59.49~($\pm$1.41)  &  57.07~($\pm$3.03) & 52.92~($\pm$0.29)& 26.09~($\pm$0.23)& 39.60~($\pm$2.38)   \\
\quad Our Model & \textbf{63.45}~($\pm$0.29) &  \textbf{61.67}~($\pm$0.58)& \textbf{58.82}~($\pm$0.37)  & \textbf{
39.00}~($\pm$0.30) & \textbf{41.72}~($\pm$1.18)  \\
\hline

BART$_\text{large}$ \\
\quad Text2Text$_\text{vanilla}$ & 66.91~($\pm$2.14)&  61.46~($\pm$1.74)  & 62.81~($\pm$2.15) & 28.55~($\pm$4.97)  & 47.80~($\pm$2.22)  \\

\quad Text2Text$_\text{Enc}$ & 67.35~($\pm$0.90)&  62.47~($\pm$1.53)  & 65.33~($\pm$1.74) & 31.13~($\pm$5.86)  & 47.19~($\pm$0.71)  \\

\quad Our Model  & \textbf{72.26}~($\pm$0.70)&  \textbf{68.07}~($\pm$1.70)  & \textbf{68.68}~($\pm$0.34)  & \textbf{45.52}~($\pm$1.54)& \textbf{55.90}~($\pm$0.92)  \\
\hline

T5$_\text{large}$ \\
\quad Text2Text$_\text{vanilla}$  & 70.63~($\pm$0.74) &  63.53~($\pm$1.10)& 62.55~($\pm$0.54) & 42.83~($\pm$2.00) & 57.74~($\pm$0.82)  \\

\quad Text2Text$_\text{Enc}$ & 70.30~($\pm$0.82)&  63.67~($\pm$0.46) & 66.65~($\pm$0.34)  & 28.76~($\pm$4.85) & 55.65~($\pm$0.45)   \\

\quad Our Model & \textbf{72.67}~($\pm$1.02)  &  \textbf{66.87}~($\pm$1.33) & \textbf{69.01}~($\pm$1.97)  & \textbf{47.41}~($\pm$2.00)  & \textbf{58.06}~($\pm$0.92)  \\
\hline
\end{tabular}
$}

\caption{Improvements to the Text-to-Text model.}
\label{table:comp_t2t_model}
\end{table}

\begin{table}[t!]
\centering
% \small
\resizebox{\columnwidth}{!}{$
% \resizebox{\columnwidth}{!}{$
\begin{tabular}{cccccc}
\hline
& \multicolumn{1}{c}{CSQA} & \multicolumn{1}{c}{OBQA} & \multicolumn{1}{c}{ARC-Easy} & \multicolumn{1}{c}{ARC-Challenge} & \multicolumn{1}{c}{QASC} \\
\cline{2-11}
\hline
BART$_\text{base}$ \\
\quad Our Model& \textbf{56.40}~($\pm$0.61)  &  \textbf{57.53}~($\pm$2.91)  & \textbf{56.80}~($\pm$0.28) & \textbf{33.82}~($\pm$1.66)  & \textbf{35.96}~($\pm$1.70) \\
\quad w/o gen loss  & 54.35~($\pm$1.97)&  54.27~($\pm$0.92)& 55.42~($\pm$1.26) & 32.62~($\pm$0.31) & 25.99~($\pm$0.82)  \\  
\quad Pipeline Clue & 46.41~($\pm$1.79)    & 52.93~($\pm$1.1)  & 48.87~($\pm$1.29)  & 27.64~($\pm$0.69)   & 21.31~($\pm$1.03)  \\  
% \quad w/o clue& 54.30~($\pm$0.83)&  53.60~($\pm$2.62) & 54.90~($\pm$0.58) & 32.27~($\pm$0.26)  & 26.67~($\pm$0.71)  \\  
\hline

T5$_\text{base}$ \\
\quad Our Model& \textbf{63.45}~($\pm$0.29)&  \textbf{61.67}~($\pm$0.58)& \textbf{58.82}~($\pm$0.37)  & \textbf{
39.00}~($\pm$0.30) & \textbf{41.72}~($\pm$1.18)  \\
\quad w/o gen loss & 60.88~($\pm$1.89) &  59.73~($\pm$0.90) & 57.10~($\pm$0.72)& 37.54~($\pm$0.64) & 36.29~($\pm$1.66)  \\  
\quad Pipeline Clue  & 48.79~($\pm$0.87) & 54.93~($\pm$1.63)  & 46.65~($\pm$0.54) & 26.01~($\pm$1.28)  & 27.50~($\pm$1.56)  \\  
% \quad w/o clue & 59.05~($\pm$0.71) &  58.27~($\pm$2.05) & 56.84~($\pm$1.78)  & 36.25~($\pm$1.73) & 36.36~($\pm$0.92)  \\  
\hline

BART$_\text{large}$ \\
\quad Our Model & \textbf{72.26}~($\pm$0.70) &  \textbf{68.07}~($\pm$1.70) & \textbf{68.68}~($\pm$0.34) & \textbf{45.52}~($\pm$1.54)& \textbf{55.90}~($\pm$0.92)  \\
\quad w/o gen loss & 69.64~($\pm$2.76)&  64.47~($\pm$1.40)  & 65.71~($\pm$1.4 & 24.92~($\pm$2.06) & 52.02~($\pm$1.44)  \\  
\quad Pipeline Clue  & 55.23~($\pm$0.62)   & 59.20~($\pm$0.69)  & 54.22~($\pm$1.27)   & 37.60~($\pm$0.90)   & 32.47~($\pm$1.11)  \\  
% \quad w/o clue    & 71.61~($\pm$1.07) &  65.40~($\pm$1.39)& 67.04~($\pm$0.69) & 42.63~($\pm$1.01)  & 51.94~($\pm$1.31)  \\  
\hline

T5$_\text{large}$ \\
\quad Our Model& \textbf{72.67}~($\pm$1.02) &  \textbf{66.87}~($\pm$1.33) & \textbf{69.01}~($\pm$1.97) & \textbf{47.41}~($\pm$2.00)  & \textbf{58.06}~($\pm$0.92)  \\
\quad w/o gen loss  & 71.66~($\pm$1.28)&  65.87~($\pm$0.90) & 66.24~($\pm$0.79)  & 46.24~($\pm$1.29) & 53.35~($\pm$1.35)  \\ 
\quad Pipeline Clue& 60.74~($\pm$0.29)   & 57.73~($\pm$1.1)   & 48.36~($\pm$2.15)  & 30.50~($\pm$1.46)    & 38.77~($\pm$1.74)  \\ 
% \quad w/o clue & 70.52~($\pm$0.22)&  66.20~($\pm$0.72)& 66.19~($\pm$3.40)  & 43.23~($\pm$0.95)& 51.98~($\pm$1.68)   \\
\hline
\end{tabular}
$}
\caption{Influence of Clue.}
\label{table:wo_clue}
\end{table}
